# Supplementary material for: Impact of spatially correlated pore-scale heterogeneity on drying porous media
Source: arXiv:1612.01032 source file (2017-05-03)
Supplement: Supplementary file 1 [file Supp_Info_Borgman_2016WR020260_R1.pdf]

# Supporting Information for
# "Impact of spatially correlated pore-scale heterogeneity on drying porous media"

**Oshri Borgman,[1] Paolo Fantinel,[2] Wieland Lühder,[2] Lucas Goehring[2,3], and Ran Holtzman[1]**

[1]Department of Soil and Water Sciences, The Hebrew University of Jerusalem, Rehovot 7610001, Israel

[2]Max Planck Institute for Dynamics and Self-Organization (MPIDS), 37077 Göttingen, Germany

[3]School of Science and Technology, Nottingham Trent University, Clifton Lane, Nottingham, NG11 8NS, UK

## Introduction

This document includes (i) details of the derivation of Eq. (3) in the main text; (ii) example of vapor saturation profiles showing the two-dimensional structures that develops in the boundary layer; (iii) the complete set of drying patterns (at breakthrough) and drying curves (rate vs. saturation) from all microfluidic experiments with corresponding simulated patterns; and (iv) videos highlighting the dynamic evolution of the drying pattern in experiments and simulations.

## (i) Derivation of the Liquid Volume-Meniscus Curvature Relationship

Our pore-scale model includes capillary invasion of air, once the critical entry threshold has been exceeded. At each time step, we update the capillary pressures (or equivalently, the meniscus curvature $C$, where the two are related via the Young-Laplace law) in each pore throat $ij$ according to the amount of liquid evaporated during that step, $\Delta V_{ij}$. To relate the change in curvature to changes in liquid volume, we approximating each throat as a cylindrical capillary tube with an effective radius of $r^*_{ij} = \left(1/h + 1/w_{ij}\right)^{-1}$ (Fig. S1), where $w_{ij}$ is the throat aperture and $h$ is the pillar height (out of plane sample thickness). This allows consideration of a spherical meniscus of curvature $C$, and predict the onset of capillary invasion once the critical curvature for throat $ij$, $C^*_{ij} = 2/r^*_{ij}$, has been exceeded, $C \geq C^*_{ij}$.

With the above, the volume evaporated from the meniscus $\Delta V_{ij}$ (measured since the initial condition of zero curvature, $C = 0$) is related to its current curvature $C = 2/R$ ($R$ be-

Corresponding author: Ran Holtzman, holtzman.ran@mail.huji.ac.il

ing its radius of curvature, the sphere radius in Fig. S1), through the spherical cap equation,

$$\Delta V_{ij} = \frac{\pi b^2}{3}(3R - b) \tag{1}$$

where $b = R(1 - \sin\alpha)$ is the cap height and $\alpha = \cos^{-1}\left(r^*_{ij}/R\right)$. Replacing the current and critical radii with their equivalent curvatures, $C$ and $C^*_{ij}$ with some rearrangements leads to Eq. (3) in the main text, which relates changes in liquid volume to meniscus curvature, or equivalently, capillary pressure.

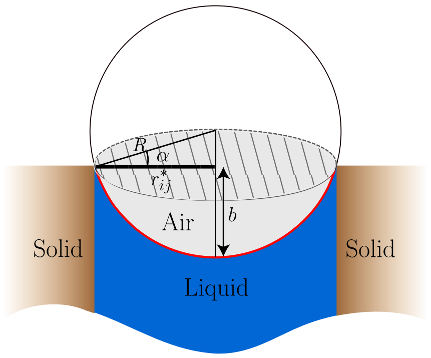


**Figure S1.** Schematics of our model relating the air-liquid meniscus curvature to the amount of liquid evaporated. A throat $ij$ is represented as a cylindrical capillary tube with an effective radius of $r^*_{ij}$, with a spherical meniscus (red line) of curvature $C = 2/R$ where $R$ is its radius of curvature. The volume evaporated since initial condition of zero curvature ($C = 0$), $\Delta V_{ij}$, is the volume of the spherical cap (gray shading).

### (ii) Vapor concentration profiles in the boundary layer

The atmospheric demand of vapor, which sets the potential rate of evaporation from the porous media, is controlled by vapor diffusion in the air boundary layer that forms above the medium's open surface. We extend here our model to include calculation of the vapor concentrations and fluxes in the boundary layer, by discretizing the boundary layer into a network of interconnected cells. This captures the coupling between the porous media and the boundary layer, namely the surface-wetness dependent distribution of vapor concentration. As a pore on the sample surface is invaded, its vapor flux decreases and allows the vapor flux of an adjacent wet pore to increase, due to horizontal (parallel to the surface) vapor diffusion [*Shahraeeni et al.*, 2012]. Few examples of vapor concentration distributions (for a specific simulation at different values of $S_{\mathrm{surf}}$) in Fig. S2 demonstrate the 2-D nature of the concentration profile.

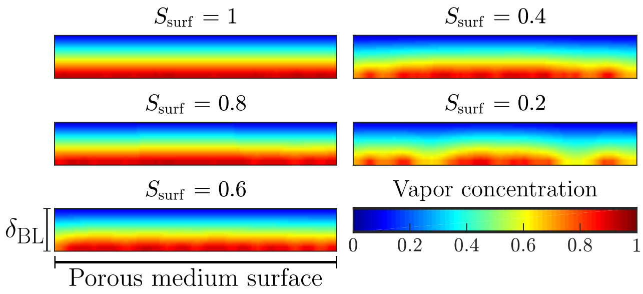


**Figure S2.** Vapor concentrations over the surface of the sample are plotted for various surface saturation $S_{\mathrm{surf}}$, showing the gradual transition from a 1-D concentration profile for high $S_{\mathrm{surf}}$ to a 2-D distribution at low $S_{\mathrm{surf}}$, driven by lateral diffusion of vapor in the boundary layer. The location of the porous medium surface and the boundary layer, (width $\delta_{\mathrm{BL}}$), are indicated only on the panel with $S_{\mathrm{surf}} = 0.6$. Porous media itself not shown.

## (iii) Comparison of Experimental and Simulated Patterns

For completeness, we provide in Fig. S3 the entire set of drying patterns (at breakthrough) from all microfluidic experiments, alongside with the corresponding simulated patterns (for similar pore geometry). In addition, we plot the drying rates versus liquid saturation. Data shown here includes 8 experiments with no spatial correlation ($\zeta = 0$, Fig. S3) and 14 experiments with correlated porous media ($\zeta > 0$, Fig. S3 contd.). The data set for $\zeta = 0$ includes four $\lambda$ values, with two experimental realizations (different random pillar sizes) for each combination of $\zeta$ and $\lambda$ (total of 8 different sample designs). For the correlated samples, data includes two disorder values ($\lambda$=0.1, and 0.2) and four correlation values ($\zeta$=1, 4, 10 and 15), again totaling 8 sample designs. For $\zeta$ of 1, 4, $\lambda$=0.1, and $\zeta$=15, $\lambda$=0.2, experiments were repeated three times using samples with similar sample design (made from the same mold), albeit with small differences due to manufacturing errors. As these errors are small (~1.6 $\mu$m in pillar size, ~3.2% of design), the difference between emergent patterns demonstrate the sensitivity of the patterns to small details, where slight changes in pore sizes, even locally, can significantly alter the pattern. We provide the match in patterns for each pair of experimental and simulated pattern, computed from the number of *overlapping* invaded pores (in both) divided by the average number of invaded pores, at breakthrough. For each realization we also show the pore sizes (the volume between four adjacent solid pillars), normalized by the mean pore size.

An extreme case of the experimental sensitivity to small manufacturing errors is exemplified by the distinctively different patterns for $\lambda = 0.2$, $\zeta = 15$. We believe that the reason lies in a "binary choice" occurring when the invasion front reaches a bottleneck (a very narrow throat); when such a throat is slightly shrinked (due to manufacturing error), the invasion may proceed elsewhere, completely avoiding an entire region. Another variation within experiments of similar design is their initial drying rate, which were not effectively set by the designed boundary layer in the microfluidic cell (the empty region without pillars near the open end of the cell, see Section 2 of the main text for details). This uncertainty in the thickness of the actual boundary layer that formed outside the porous medium is believed to be a consequence of bending of the substrate, as well as by potential extension of the boundary layer outside the manufactured cell. In the simulations which are compared with the experiments, we use in an effective value for $\delta_{\mathrm{BL}}$, computed by matching the initial experimental rates.

### (iv) Videos showing dynamics of pattern evolution

Here, we compare the evolution of the experimental and simulated drying pattern via a pair of videos, Borgman-ms01 and Borgman-ms02, respectively (for $\zeta = 4$). The videos emphasize the main difference: isolated clusters in the simulations tend to dry out faster than in the experiments, as reflected in the evolution of Euler number. The disappearance of isolated liquid clusters reduces the wetness near the surface and advances the air-liquid interface deeper into the porous medium, resulting in a notable decrease in drying rates.

## References

Shahraeeni, E., P. Lehmann, and D. Or (2012), Coupling of evaporative fluxes from drying porous surfaces with air boundary layer: Characteristics of evaporation from discrete pores, *Water Resour. Res.*, *48*(9), W09,525, doi:10.1029/2012WR011857.

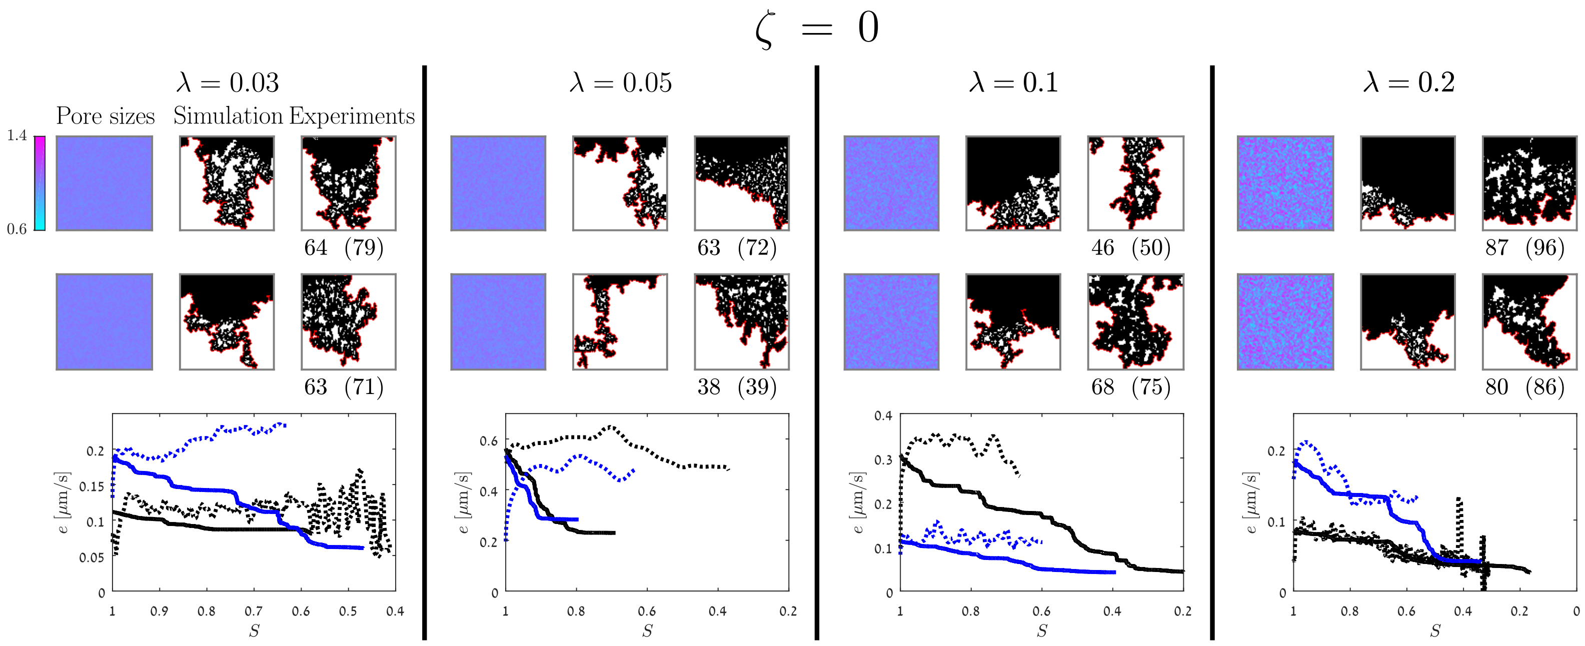


**Figure S3.** Pore size distribution, simulated and experimental drying patterns at breakthrough, and match in patterns (in %, parentheses provide match considering only the leading front), for $\zeta$=0 and various $\lambda$ values. In the patterns, black and white represent dry and wet pores (solid not shown); red line shows the invasion front. Experimental and simulated drying curves (rates vs. liquid saturation) are plotted in dotted and solid lines, respectively. Black and blue lines correspond to the upper and lower sample (which has different random seed, same $\zeta$ and $\lambda$).

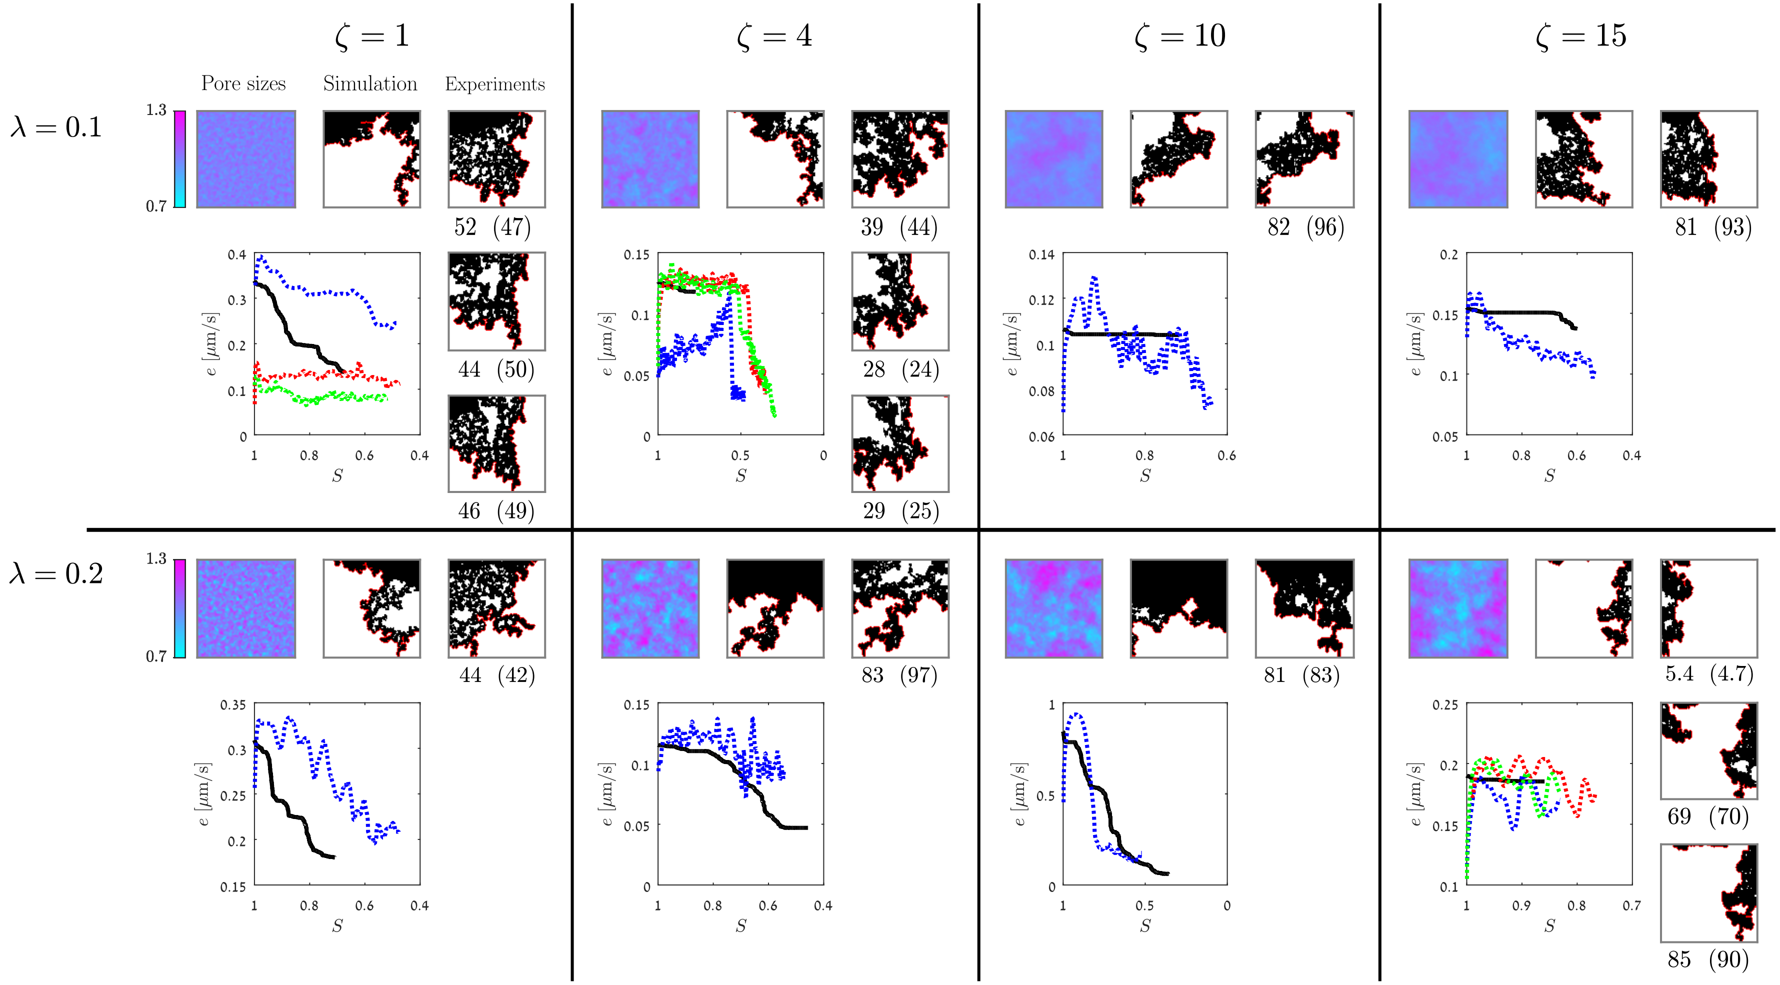


**Figure S3. (continued)** Pore size distribution, simulated and experimental drying patterns at breakthrough, and match in patterns (in %, parentheses provide match considering only the leading front), for $\zeta$= 1, 4, 10, and 15 and various $\lambda$. Black and white represent dry and wet pores (solid not shown); red line shows the invasion front. Experimental and simulated drying curves (rates vs. liquid saturation): in cases where several experimental runs were made on the same sample design, blue, red and green dotted lines correspond to the patterns of the upper, middle and lower experimental runs. Black solid line corresponds to the simulated rate, using an effective boundary layer that was evaluated from the upper experimental run.
